# Supplementary material for: Aufbau suppressed coupled cluster as a post-linear-response method
Source: arXiv:2506.16680 source file (2025-06-20)
Supplement: Supplementary file 1 [file SI_allResults.pdf]

| | Molecule | State | Flip | Rydberg | REF | *n*-CSF | | | | Excitation energy (eV) | | | | ASCC excitation energy (eV) | | | | | | | | PLASCC excitation energy (eV) | | | | | | | |
|---|---|---|---|---|---|---|---|---|---|---|---|---|---|---|---|---|---|---|---|---|---|---|---|---|---|---|---|---|---|
| | | | | | | *ESMF* | *CIS* | *wB97X-V* | *EOM-CCSD* | *ESMF* | *CIS* | *wB97X-V* | *EOM-CCSD* | *ESMF* | | *CIS* | | *wB97X-V* | | *EOM-CCSD* | | *ESMF* | | *CIS* | | *wB97X-V* | | *EOM-CCSD* | |
| Small QUEST set | H2O | 11B1 | | R | 7.53 | 1 | 1 | 1 | 1 | 6.46 | 8.67 | 7.29 | 7.45 | 7.50 | 7.50 | 7.54 | 7.54 | 7.54 | 7.54 | 7.53 | 7.53 | 7.51 | 7.51 | 7.52 | 7.52 | 7.50 | 7.50 | 7.49 | 7.49 |
| | H2O | 11A2 | | R | 9.32 | 1 | 1 | 1 | 1 | 8.13 | 10.35 | 8.90 | 9.21 | 9.27 | 9.27 | 9.33 | 9.33 | 9.32 | 9.32 | 9.30 | 9.30 | 9.28 | 9.28 | 9.29 | 9.29 | 9.28 | 9.28 | 9.27 | 9.27 |
| | H2O | 21A1 | Y | R | 9.94 | 1 | 1 | 1 | 1 | 8.87 | 11.00 | 9.52 | 9.86 | 9.86 | 9.94 | 9.87 | 10.03 | 10.04 | 9.87 | 9.96 | 9.91 | 9.90 | 9.92 | 9.87 | 9.94 | 9.95 | 9.86 | 9.89 | 9.89 |
| | H2S | 11B1 | | R | 6.10 | 1 | 1 | 1 | 1 | 5.75 | 6.59 | 6.24 | 6.13 | 6.12 | 6.12 | 6.12 | 6.12 | 6.13 | 6.13 | 6.13 | 6.13 | 6.11 | 6.11 | 6.10 | 6.10 | 6.11 | 6.11 | 6.11 | 6.11 |
| | H2S | 11A2 | | R | 6.29 | 1 | 1 | 1 | 1 | 6.11 | 6.42 | 6.20 | 6.34 | 6.28 | 6.28 | 6.29 | 6.29 | 6.29 | 6.29 | 6.29 | 6.29 | 6.28 | 6.28 | 6.27 | 6.27 | 6.27 | 6.27 | 6.27 | 6.27 |
| | Ammonia | 11A2 | Y | R | 6.48 | 1 | 1 | 1 | 1 | 5.56 | 7.43 | 6.43 | 6.46 | 6.42 | 6.47 | 6.44 | 6.49 | 6.44 | 6.49 | 6.46 | 6.49 | 6.46 | 6.47 | 6.41 | 6.48 | 6.41 | 6.46 | 6.42 | 6.45 |
| | Ammonia | 11E | | R | 8.08 | 1 | 1 | 1 | 1 | 6.99 | 8.91 | 7.91 | 8.03 | 8.03 | 8.03 | 8.05 | 8.05 | 8.05 | 8.05 | 8.05 | 8.05 | 8.06 | 8.06 | 8.04 | 8.04 | 8.03 | 8.03 | 8.03 | 8.03 |
| | Ammonia | 21A1 | Y | R | 9.68 | 1 | 1 | 1 | 1 | 8.62 | 10.46 | 9.59 | 9.65 | 9.65 | 9.42 | 9.41 | 9.72 | 9.44 | 9.72 | 9.55 | 9.64 | 9.64 | 9.57 | 9.49 | --- | 9.49 | 9.67 | 9.60 | --- |
| | Ammonia | 21A2 | Y | R | 10.41 | 1 | 1 | 1 | 1 | 9.48 | 11.30 | 10.28 | 10.38 | 10.45 | 10.21 | 10.31 | 10.41 | --- | 10.38 | --- | --- | 10.40 | 10.39 | 10.38 | 10.39 | 10.38 | 10.38 | 10.38 | 10.39 |
| | HCl | 1pi | | | 7.82 | 1 | 1 | 1 | 1 | 7.44 | 8.36 | 7.79 | 7.86 | 7.82 | 7.82 | 7.84 | 7.84 | 7.84 | 7.84 | 7.84 | 7.84 | 7.82 | 7.82 | 7.82 | 7.82 | 7.81 | 7.81 | 7.81 | 7.81 |
| | N2 | 11pig | | | 9.41 | 1 | 1 | 1 | 1 | 9.79 | 9.97 | 9.54 | 9.49 | 9.64 | 9.64 | 9.63 | 9.63 | 9.65 | 9.65 | 9.66 | 9.66 | 9.46 | 9.46 | 9.44 | 9.44 | 9.46 | --- | 9.45 | --- |
| | N2 | 11sigu- | | | 10.05 | 2 | 2 | 2 | 2 | 8.36 | 8.45 | 9.27 | 10.20 | 10.14 | 10.14 | 10.14 | 10.14 | 10.14 | 10.14 | 10.14 | 10.14 | 10.23 | 10.23 | 10.23 | 10.23 | 10.23 | 10.23 | 10.22 | 10.22 |
| | N2 | 11deltau | | | 10.43 | 2 | 2 | 2 | 2 | 8.92 | 9.01 | 9.72 | 10.61 | 10.55 | 10.55 | 10.55 | 10.55 | 10.56 | 10.56 | 10.55 | 10.55 | 10.55 | 10.55 | 10.55 | 10.55 | 10.56 | --- | 10.55 | --- |
| | CO | 11pi | | | 8.57 | 1 | 1 | 1 | 1 | 8.48 | 9.01 | 8.72 | 8.67 | 8.66 | 8.66 | 8.67 | 8.67 | 8.70 | 8.70 | 8.69 | 8.69 | 8.59 | 8.59 | 8.50 | 8.50 | 8.54 | 8.54 | 8.53 | 8.53 |
| | CO | 11sig- | | | 10.05 | 2 | 2 | 2 | 2 | 8.36 | 9.62 | 9.72 | 10.10 | 10.12 | 10.12 | 10.14 | 10.14 | 10.14 | 10.14 | 10.14 | 10.14 | 10.17 | 10.17 | 10.16 | 10.16 | 10.17 | 10.17 | 10.17 | 10.17 |
| | CO | 11del | | | 10.16 | 2 | 2 | 2 | 2 | 8.55 | 10.04 | 10.08 | 10.21 | 10.26 | 10.26 | 10.29 | 10.29 | 10.29 | 10.29 | 10.29 | 10.29 | 10.26 | 10.26 | 10.22 | 10.22 | 10.24 | 10.24 | 10.25 | 10.25 |
| | CO | 21sig+ | Y | R | 10.94 | 1 | 1 | 1 | 1 | 10.95 | 12.36 | 11.21 | 11.17 | 11.19 | 10.78 | 11.28 | 10.78 | 10.81 | 11.18 | 10.92 | 11.21 | --- | 10.88 | 11.45 | 11.24 | 10.85 | --- | 10.97 | --- |
| | CO | 31sig+ | Y | R | 11.52 | 1 | 1 | 1 | 1 | 11.26 | 12.81 | 11.43 | 11.71 | 11.48 | --- | 11.21 | 10.97 | 11.64 | 11.42 | 11.50 | 11.69 | 11.51 | 11.65 | 11.29 | 11.46 | 11.67 | 11.51 | 11.58 | 11.69 |
| | CO | 21pi | | R | 11.76 | 1 | 1 | 1 | 1 | 11.72 | 12.96 | 11.65 | 11.97 | 11.87 | 11.87 | 11.79 | 11.79 | 11.85 | 11.85 | 11.90 | 11.90 | 11.89 | 11.89 | 11.77 | 11.77 | 11.85 | --- | 11.89 | --- |
| | Acetylene | 11sigu- | | | 7.20 | 2 | 2 | 2 | 2 | 6.12 | 6.28 | 6.85 | 7.27 | 7.28 | 7.28 | 7.29 | 7.29 | 7.29 | --- | 7.28 | --- | 7.34 | 7.34 | 7.34 | 7.34 | 7.35 | --- | 7.34 | --- |
| | Acetylene | 11delu | | | 7.51 | 2 | 2 | 2 | 2 | 6.42 | 6.62 | 6.84 | 7.57 | 7.59 | 7.59 | 7.60 | 7.60 | 7.60 | --- | 7.60 | --- | 7.64 | 7.64 | 7.61 | 7.61 | 7.63 | --- | 7.64 | 7.64 |
| | Ethylene | 11B3u | | R | 7.31 | 1 | 1 | 1 | 1 | 6.06 | 7.15 | 7.22 | 7.33 | 7.22 | 7.22 | 7.22 | 7.22 | 7.23 | 7.23 | 7.24 | 7.24 | 7.31 | 7.31 | 7.29 | 7.29 | 7.30 | 7.30 | 7.30 | 7.30 |
| | Ethylene | 11B1u | | | 7.93 | 1 | 1 | 1 | 1 | 7.24 | 7.74 | 7.99 | 8.04 | 7.88 | 7.88 | 7.87 | 7.87 | 7.88 | 7.88 | 7.89 | 7.89 | 7.88 | 7.88 | 7.88 | 7.88 | 7.89 | 7.89 | 7.91 | 7.90 |
| | Ethylene | 11B1g | | R | 8.00 | 1 | 1 | 1 | 1 | 6.70 | 7.76 | 7.88 | 8.01 | 7.91 | 7.91 | 7.91 | 7.91 | 7.92 | 7.92 | 7.92 | 7.92 | 8.00 | 8.00 | 7.98 | 7.98 | 8.00 | 8.00 | 8.00 | 8.00 |
| | Formaldehyde | 11A2 | | | 3.99 | 1 | 1 | 1 | 1 | 3.09 | 4.55 | 3.98 | 4.02 | 3.95 | 3.95 | 4.05 | 4.05 | 4.07 | 4.07 | 4.07 | 4.07 | 3.95 | 3.95 | 3.94 | 3.94 | 3.94 | 3.94 | 3.92 | 3.92 |
| | Formaldehyde | 11B2 | | R | 7.11 | 1 | 1 | 1 | 1 | 6.26 | 8.57 | 7.11 | 7.04 | 7.11 | 7.11 | 7.21 | 7.21 | 7.21 | 7.21 | 7.19 | 7.19 | 7.09 | 7.09 | --- | 7.16 | --- | --- | 7.10 | 7.10 |
| | Formaldehyde | 21B2 | | R | 8.04 | 1 | 1 | 1 | 1 | 7.30 | 9.44 | 8.02 | 7.99 | 8.08 | 8.08 | 8.18 | 8.18 | 8.19 | 8.19 | 8.15 | 8.15 | 8.05 | 8.05 | 8.06 | 8.06 | 8.08 | 8.08 | 8.08 | 8.08 |
| | Formaldehyde | 21A2 | | R | 8.65 | 1 | 1 | 1 | 1 | 8.00 | 10.19 | 8.61 | 8.61 | 8.72 | 8.72 | 8.78 | 8.78 | 8.78 | 8.78 | 8.77 | 8.77 | 8.69 | 8.69 | 8.69 | 8.69 | 8.72 | 8.72 | 8.70 | 8.70 |
| | Formaldehyde | 11B1 | | | 9.29 | 1 | 1 | 1 | 1 | 8.35 | 9.87 | 9.28 | 9.37 | 9.27 | 9.27 | 9.37 | 9.37 | 9.39 | 9.39 | 9.38 | 9.38 | 9.27 | 9.27 | 9.30 | 9.30 | 9.32 | 9.32 | 9.31 | 9.31 |
| | Thioformaldehyde | 11A2 | | | (a)2.26 | 1 | 1 | 1 | 1 | 1.54 | 2.69 | 2.27 | 2.32 | 2.16 | 2.16 | 2.25 | 2.25 | 2.26 | 2.26 | 2.27 | 2.27 | 2.23 | 2.23 | 2.13 | 2.13 | 2.14 | 2.14 | 2.11 | 2.11 |
| | Thioformaldehyde | 11B2 | | R | 5.83 | 1 | 1 | 1 | 1 | 5.29 | 6.53 | 6.14 | 5.84 | 5.85 | 5.85 | 5.89 | 5.89 | 5.90 | 5.90 | 5.89 | 5.89 | 5.83 | 5.83 | 5.77 | 5.77 | 5.81 | 5.81 | 5.85 | 5.85 |
| | Thioformaldehyde | 21A1 | Y | | 6.51 | 1 | 1 | 2 | 2 | 6.30 | 6.42 | 6.77 | 6.75 | 6.61 | 6.74 | 6.64 | 6.68 | 6.62 | 6.57 | 6.55 | 6.68 | 6.74 | 6.50 | 6.54 | 6.73 | 6.69 | 6.62 | 6.59 | 6.76 |
| | Methanimine | 11Ad | | | 5.25 | 1 | 1 | 1 | 1 | 4.53 | 5.86 | 5.28 | 5.31 | 5.22 | 5.22 | 5.32 | 5.32 | 5.33 | 5.33 | 5.33 | 5.33 | 5.23 | 5.23 | 5.16 | 5.16 | 5.18 | 5.18 | 5.16 | 5.16 |
| | Acetaldehyde | 11Ad | | | 4.34 | 1 | 1 | 1 | 1 | 4.38 | 4.98 | 4.35 | 4.36 | 4.30 | 4.30 | 4.40 | 4.40 | 4.43 | 4.43 | 4.42 | 4.42 | 4.28 | 4.28 | 4.27 | 4.27 | 4.28 | 4.28 | 4.26 | 4.26 |
| | Cyclopropene | 11B1 | | | (b)6.71 | 1 | 2 | 1 | 1 | 6.37 | 7.23 | 6.59 | 6.78 | 6.77 | 6.77 | 6.82 | 6.82 | 6.79 | 6.79 | 6.80 | 6.80 | 6.74 | 6.74 | *6.75 | --- | 6.71 | 6.71 | 6.70 | 6.70 |
| | Cyclopropene | 11B2 | | | 6.82 | 1 | 1 | 1 | 1 | 6.48 | 6.74 | 6.67 | 6.88 | 6.86 | 6.86 | 6.86 | 6.86 | 6.88 | 6.88 | 6.87 | 6.87 | 6.78 | 6.78 | 6.78 | 6.78 | 6.80 | 6.80 | 6.79 | 6.79 |
| | Diazomethane | 11A2 | | | 3.09 | 1 | 1 | 1 | 1 | 2.11 | 3.14 | 3.05 | 3.23 | 2.97 | 2.97 | 3.06 | 3.06 | 3.04 | 3.04 | 3.04 | 3.04 | 3.06 | 3.06 | 2.82 | 2.82 | 2.88 | 2.88 | 2.86 | 2.86 |
| | Diazomethane | 11B1 | | R | 5.35 | 1 | 1 | 1 | 1 | 4.87 | 5.70 | 5.53 | 5.43 | 5.31 | 5.31 | 5.29 | 5.29 | 5.32 | 5.32 | 5.33 | 5.33 | 5.34 | 5.34 | 5.33 | 5.33 | 5.37 | 5.37 | 5.37 | 5.37 |
| | Diazomethane | 21A1 | Y | | 5.79 | 1 | 1 | 2 | 1 | 5.71 | 6.23 | 6.10 | 5.90 | 5.84 | 5.90 | 5.80 | 5.93 | 5.90 | 5.83 | 5.90 | 5.90 | 5.81 | 5.56 | 5.75 | 5.76 | 5.88 | 5.68 | 5.82 | 5.77 |
| | Formamide | 11A'' | | | 5.70 | 1 | 1 | 1 | 1 | 4.69 | 6.52 | 5.68 | 5.71 | 5.62 | 5.62 | 5.73 | 5.73 | 5.75 | 5.75 | 5.74 | 5.74 | 5.60 | 5.60 | 5.55 | 5.55 | 5.58 | 5.58 | 5.55 | 5.55 |
| | Formamide | 21A' | Y | R | 6.67 | 1 | 2 | 2 | 2 | 5.87 | 8.53 | 7.11 | 6.83 | 6.73 | 6.84 | 7.00 | 6.83 | 6.86 | 6.82 | 6.82 | 6.79 | 6.78 | 6.76 | --- | *6.84 | *6.99 | *7.02 | *6.85 | --- |
| | Formamide | 31A' | Y | | 7.64 | 2 | 1 | 2 | 2 | 8.02 | 9.43 | 8.29 | 7.72 | 7.84 | 7.90 | 7.35 | 7.44 | 7.79 | 7.82 | 7.95 | 7.95 | *7.70 | *7.33 | 7.31 | 7.45 | --- | --- | *7.48 | *7.57 |
| | Formamide | 41A' | Y | R | 7.29 | 1 | 2 | 2 | 2 | 6.45 | 8.91 | 7.63 | 7.41 | 7.40 | 7.36 | 7.86 | 7.87 | 7.41 | 7.41 | *7.47 | *7.45 | 7.37 | 7.36 | --- | *7.37 | *7.28 | *7.23 | *7.28 | *7.31 |
| | Ketene | 11A2 | | | 3.84 | 1 | 1 | 1 | 1 | 3.38 | 4.31 | 3.94 | 3.97 | 3.84 | 3.84 | 3.88 | 3.88 | 3.91 | 3.91 | 3.92 | 3.92 | 3.82 | 3.82 | 3.74 | 3.74 | 3.79 | 3.79 | 3.77 | 3.77 |

| Molecule | State | Flip | Rydberg | REF | *n*-CSF | | | | Excitation energy (eV) | | | | ASCC excitation energy (eV) | | | | | | | | PLASCC excitation energy (eV) | | | | | | | |
|---|---|---|---|---|---|---|---|---|---|---|---|---|---|---|---|---|---|---|---|---|---|---|---|---|---|---|---|---|
| | | | | | *ESMF* | *CIS* | *wB97X-V* | *EOM-CCSD* | *ESMF* | *CIS* | *wB97X-V* | *EOM-CCSD* | *ESMF* | | *CIS* | | *wB97X-V* | | *EOM-CCSD* | | *ESMF* | | *CIS* | | *wB97X-V* | | *EOM-CCSD* | |
| Ketene | 11B1 | | R | 5.88 | 1 | 1 | 1 | 1 | 5.55 | 6.42 | 6.06 | 5.94 | 5.93 | 5.93 | 5.90 | 5.90 | 5.96 | 5.96 | 5.97 | 5.97 | 5.92 | 5.92 | 5.88 | 5.88 | 5.96 | 5.96 | 5.97 | 5.97 |
| Ketene | 21A2 | | R | 7.08 | 1 | 1 | 1 | 1 | 6.52 | 7.53 | 7.20 | 7.15 | 7.10 | 7.10 | 7.08 | 7.08 | 7.13 | 7.13 | 7.15 | 7.15 | --- | *7.13 | 7.10 | 7.10 | 7.18 | 7.18 | 7.18 | 7.18 |
| Nitrosomethane | 11A" | | | 1.99 | 1 | 1 | 1 | 1 | 2.35 | 2.08 | 1.91 | 2.00 | 2.04 | 2.04 | 2.09 | 2.09 | 2.11 | 2.11 | 2.10 | 2.10 | 2.02 | 2.02 | 2.00 | 2.00 | 2.03 | 2.03 | 2.01 | 2.01 |
| Streptocyanine-C1 | 11B2 | | | 7.14 | 1 | 1 | 1 | 1 | 7.26 | 8.55 | 7.94 | 7.22 | 7.19 | 7.19 | 7.22 | 7.22 | 7.25 | 7.25 | 7.25 | 7.25 | 7.12 | 7.12 | 7.01 | 7.01 | 7.01 | 7.01 | 7.01 | 7.01 |
| acetone | 11A2 | | | 4.48 | 1 | 1 | 1 | 1 | 3.67 | 5.23 | 4.54 | 4.53 | 4.47 | 4.47 | 4.58 | 4.58 | 4.61 | 4.61 | 4.60 | 4.60 | 4.44 | 4.44 | 4.42 | 4.42 | 4.45 | 4.45 | 4.42 | 4.42 |
| acetone | 11B2 | | R | 6.30 | 1 | 1 | 1 | 1 | 5.76 | 8.26 | 6.73 | 6.40 | 6.47 | 6.47 | 6.56 | 6.56 | 6.57 | 6.57 | 6.55 | 6.55 | 6.39 | 6.39 | 6.77 | --- | 6.38 | 6.38 | 6.43 | 6.43 |
| acetone | 21A1 | Y | | 7.36 | 1 | 2 | 1 | 1 | 6.60 | 9.24 | 7.80 | 7.46 | 7.52 | 7.49 | 7.53 | 7.62 | 7.55 | 7.68 | 7.58 | 7.61 | 7.42 | 7.53 | 7.43 | 7.43 | 7.39 | 7.44 | 7.53 | *7.47 |
| acetone | 21A2 | | R | 7.38 | 1 | 1 | 1 | 1 | 6.61 | 9.21 | 7.78 | 7.43 | 7.49 | 7.49 | 7.58 | 7.58 | 7.58 | 7.58 | 7.57 | 7.57 | 7.44 | 7.44 | 7.43 | 7.43 | 7.49 | 7.49 | 7.49 | 7.49 |
| acetone | 21B2 | | R | 7.55 | 1 | 1 | 1 | 1 | 6.80 | 9.34 | 7.88 | 7.60 | 7.67 | 7.67 | 7.80 | 7.80 | 7.81 | 7.81 | 7.75 | 7.75 | 7.62 | 7.62 | 7.59 | 7.59 | 7.65 | 7.65 | 7.68 | 7.68 |
| isobutene | 11B1 | | | 6.39 | 1 | 1 | 1 | 1 | 5.43 | 6.63 | 6.52 | 6.44 | 6.41 | 6.41 | 6.41 | 6.41 | 6.43 | 6.43 | 6.43 | 6.43 | 6.44 | 6.44 | 6.38 | 6.38 | --- | --- | *6.47 | *6.47 |
| isobutene | 21A1 | Y | | 7.00 | 1 | 1 | 1 | 1 | 6.14 | 7.13 | 7.10 | 7.06 | 7.07 | 7.00 | 6.99 | 7.01 | 7.02 | 7.04 | 7.07 | 6.99 | 7.06 | 6.93 | 6.93 | 7.04 | 6.96 | 7.08 | 7.10 | 6.92 |
| thioacetone | 11A2 | | | 2.57 | 1 | 1 | 1 | 1 | 1.92 | 3.23 | 2.68 | 2.65 | 2.48 | 2.48 | 2.57 | 2.57 | 2.60 | 2.60 | 2.61 | 2.61 | 2.52 | 2.52 | 2.42 | 2.42 | 2.44 | 2.44 | 2.40 | 2.40 |
| thioacetone | 11B2 | | | 5.43 | 1 | 1 | 1 | 1 | 5.00 | 6.37 | 5.93 | 5.52 | 5.52 | 5.52 | 5.57 | 5.57 | 5.59 | 5.59 | 5.56 | 5.56 | 5.48 | 5.48 | 5.30 | 5.30 | 5.41 | 5.41 | 5.50 | 5.50 |
| thioacetone | 21A1 | Y | | 5.98 | 1 | 1 | 2 | 2 | 6.22 | 6.20 | 6.20 | 6.07 | 5.94 | 6.18 | 6.11 | 5.93 | 6.03 | 6.14 | 5.99 | 6.16 | 6.04 | 5.88 | 6.08 | 5.86 | --- | --- | *5.95 | 6.18 |
| thioacetone | 21B2 | | | 6.44 | 1 | 1 | 1 | 1 | 5.88 | 7.07 | 6.74 | 6.50 | 6.55 | 6.55 | 6.66 | 6.66 | 6.64 | 6.64 | 6.54 | 6.54 | 6.42 | 6.42 | 6.58 | 6.58 | 6.62 | 6.62 | 6.51 | 6.51 |
| thioacetone | 31A1 | Y | | 6.53 | 1 | 1 | 1 | 2 | 5.74 | 7.37 | 7.04 | 6.61 | 6.51 | 6.50 | 6.59 | 6.49 | 6.52 | 6.62 | *6.64 | 6.69 | 6.55 | 6.44 | 6.40 | 6.41 | 6.41 | 6.46 | *6.68 | *6.70 |
| cyanoformaldehyde | 11A" | | | 3.84 | 1 | 1 | 1 | 1 | 2.89 | 4.53 | 3.89 | 3.94 | 3.82 | 3.82 | 3.94 | 3.94 | 3.99 | 3.99 | 3.97 | 3.97 | 3.79 | 3.79 | 3.72 | 3.72 | 3.77 | 3.77 | 3.71 | 3.71 |
| cyanoformaldehyde | 21A" | | | 6.54 | 1 | 1 | 1 | 1 | 5.36 | 6.14 | 5.97 | 6.77 | 6.56 | 6.56 | 6.63 | 6.63 | 6.60 | 6.60 | 6.61 | 6.61 | 6.49 | 6.49 | 6.32 | 6.32 | 6.52 | 6.52 | 6.50 | 6.50 |
| propynal | 11A" | | | 3.82 | 1 | 1 | 1 | 1 | 2.94 | 4.63 | 3.92 | 3.93 | 3.80 | 3.80 | 3.92 | 3.92 | 3.95 | 3.95 | 3.95 | 3.95 | 3.76 | 3.76 | 3.67 | 3.67 | 3.70 | 3.70 | 3.66 | 3.66 |
| propynal | 21A" | | | 5.62 | 1 | 1 | 1 | 1 | 4.69 | 5.30 | 5.05 | 5.77 | 5.43 | 5.43 | 5.62 | 5.62 | 5.65 | 5.65 | 5.67 | 5.67 | 5.57 | 5.57 | 5.42 | 5.42 | 5.53 | 5.53 | 5.54 | 5.54 |
| thiopropynal | 11A" | | | 2.06 | 1 | 1 | 1 | 1 | 1.39 | 2.59 | 2.15 | 2.17 | 1.96 | 1.96 | 2.06 | 2.06 | 2.09 | 2.09 | 2.10 | 2.10 | 2.00 | 2.00 | 1.85 | 1.85 | 1.87 | 1.87 | 1.82 | 1.82 |
| cyclopropenone | 11B1 | | | 4.23 | 1 | 1 | 1 | 1 | 4.14 | 5.87 | 4.58 | 4.47 | 4.40 | 4.40 | 4.54 | 4.54 | 4.51 | 4.51 | 4.50 | 4.50 | 4.27 | 4.27 | 4.13 | 4.13 | 4.27 | 4.27 | 4.26 | 4.26 |
| cyclopropenone | 11A2 | | | 5.56 | 1 | 1 | 1 | 1 | 5.29 | 6.43 | 5.61 | 5.62 | 5.65 | 5.65 | 5.72 | 5.72 | 5.75 | 5.75 | 5.73 | 5.73 | 5.53 | 5.53 | 5.51 | 5.51 | 5.56 | 5.56 | *5.50 | *5.50 |
| cyclopropenone | 11B2 | | R | 6.19 | 1 | 2 | 1 | 1 | 5.68 | 7.76 | 6.54 | 6.27 | 6.37 | 6.37 | 6.42 | --- | 6.47 | 6.47 | 6.44 | 6.44 | 6.30 | 6.30 | 6.43 | --- | 6.47 | 6.47 | 6.39 | 6.38 |
| cyclopropenone | 31B2 | | R | 6.86 | 1 | 1 | 2 | 2 | 6.40 | 8.42 | 7.30 | 6.96 | 7.02 | 7.02 | 6.97 | 6.97 | 7.09 | --- | 7.13 | | 6.92 | 6.92 | 6.84 | 6.84 | --- | --- | *6.86 | --- |
| cyclopropenone | 21A1 | Y | R | 6.87 | 1 | 1 | 1 | 1 | 6.27 | 8.39 | 7.25 | 6.95 | 7.01 | 7.02 | 7.06 | 7.10 | 7.09 | 7.14 | 7.08 | 7.10 | 6.91 | 6.99 | 6.91 | 6.95 | 6.97 | 7.02 | 7.01 | 7.00 |
| cyclopropenone | 31A1 | Y | | 8.29 | 1 | 2 | 2 | 2 | 8.57 | 8.94 | 8.55 | 8.36 | 8.53 | 8.69 | --- | 8.40 | 8.58 | 8.64 | 8.55 | 8.62 | 8.53 | *7.87 | *8.19 | --- | *8.22 | *8.49 | *8.27 | *8.46 |
| cyclopropenethione | 11A2 | | | 3.45 | 1 | 1 | 1 | 1 | 3.22 | 4.29 | 3.57 | 3.54 | 3.44 | 3.44 | 3.50 | 3.50 | 3.53 | 3.53 | 3.53 | 3.53 | 3.40 | 3.40 | 3.34 | 3.34 | 3.36 | 3.36 | 3.34 | 3.34 |
| cyclopropenethione | 11B1 | | | 3.42 | 1 | 1 | 1 | 1 | 3.35 | 5.37 | 4.20 | 3.77 | 3.49 | 3.49 | 3.61 | 3.61 | 3.56 | 3.56 | 3.56 | 3.56 | 3.42 | 3.42 | 3.29 | 3.29 | 3.39 | 3.39 | 3.39 | 3.39 |
| cyclopropenethione | 11B2 | | | 4.64 | 1 | 1 | 1 | 1 | 4.33 | 6.24 | 5.41 | 4.95 | 4.59 | 4.59 | 4.71 | 4.71 | 4.64 | 4.64 | 4.68 | 4.67 | --- | --- | --- | --- | --- | --- | --- | --- |
| cyclopropenethione | 21B2 | | R | 5.21 | 1 | 1 | 1 | 1 | 4.67 | 5.97 | 5.71 | 5.27 | 5.27 | 5.27 | 5.32 | 5.32 | 5.35 | 5.35 | 5.31 | 5.31 | --- | --- | --- | --- | --- | --- | --- | --- |
| cyclopropenethione | 31B2 | | R | 5.84 | 1 | 1 | 1 | 1 | 5.42 | 6.87 | 6.47 | 5.93 | 5.96 | 5.96 | 5.83 | 5.83 | 5.76 | 5.76 | 5.99 | 5.99 | 5.86 | 5.86 | 6.10 | 6.10 | 6.19 | 6.19 | 5.95 | 5.95 |
| methylenecyclopropene | 11B2 | | | 4.31 | 1 | 1 | 1 | 1 | 3.69 | 5.41 | 4.84 | 4.55 | 4.25 | 4.25 | 4.37 | 4.37 | 4.30 | 4.30 | 4.35 | 4.34 | 4.30 | 4.30 | 3.79 | 3.79 | 4.04 | 4.04 | 4.04 | 4.03 |
| methylenecyclopropene | 11B1 | | R | 5.35 | 1 | 1 | 1 | 1 | 4.34 | 5.39 | 5.57 | 5.37 | 5.35 | 5.35 | 5.36 | 5.36 | 5.39 | 5.39 | 5.37 | 5.37 | 5.41 | 5.41 | 5.53 | 5.53 | 5.56 | 5.56 | 5.39 | --- |
| methylenecyclopropene | 11A2 | | R | 5.88 | 1 | 1 | 1 | 1 | 4.67 | 5.96 | 6.15 | 5.90 | 5.86 | 5.86 | 5.88 | 5.88 | 5.90 | 5.90 | 5.89 | 5.89 | 5.92 | 5.92 | 5.77 | 5.77 | *5.71 | --- | 5.93 | 5.93 |
| methylenecyclopropene | 21A1 | Y | | 6.15 | 1 | 1 | 1 | 1 | 5.42 | 6.30 | 6.40 | 6.18 | 6.21 | 6.11 | 6.15 | 6.18 | 6.21 | 6.17 | 6.17 | 6.21 | 6.20 | 6.14 | 6.02 | 6.23 | 6.27 | 6.06 | 6.08 | 6.24 |
| acrolein | 11A" | | | 3.74 | 1 | 1 | 1 | 1 | 3.16 | 4.71 | 3.90 | 3.90 | 3.78 | 3.78 | 3.91 | 3.91 | 3.94 | 3.94 | 3.93 | 3.93 | 3.68 | 3.68 | 3.52 | 3.52 | 3.58 | 3.58 | 3.55 | 3.55 |
| acrolein | 21A' | Y | | 6.70 | 1 | 1 | 2 | 2 | 6.57 | 7.05 | 6.85 | 6.86 | 6.93 | 6.91 | 7.01 | 6.89 | 6.92 | 6.99 | 7.04 | 7.07 | 6.74 | 6.81 | 6.69 | 6.27 | --- | *6.76 | *6.72 | 6.90 |
| acrolein | 31A' | Y | R | 7.00 | 1 | 1 | 1 | 2 | 6.03 | 8.77 | 7.31 | 7.11 | 7.01 | 7.01 | 7.12 | 7.15 | 7.15 | 7.16 | 7.36 | 7.34 | 6.94 | 7.03 | 7.13 | 7.22 | 7.24 | --- | --- | *7.06 |
| butadiene | 11Bu | | | 6.27 | 1 | 1 | 1 | 1 | 6.01 | 6.22 | 6.25 | 6.37 | 6.35 | 6.35 | 6.35 | 6.35 | 6.37 | 6.37 | 6.36 | 6.36 | 6.28 | 6.28 | 6.30 | 6.30 | 6.32 | 6.32 | 6.31 | 6.30 |
| butadiene | 11Bg | | R | 6.27 | 1 | 1 | 1 | 1 | 5.49 | 6.19 | 6.37 | 6.30 | 6.33 | 6.33 | 6.32 | 6.32 | 6.35 | 6.35 | 6.34 | 6.34 | 6.39 | 6.39 | 6.38 | 6.38 | 6.41 | 6.41 | 6.40 | 6.40 |
| butadiene | 21Ag | Y | | 6.59 | 1 | 1 | 1 | 2 | 6.91 | 7.41 | 7.31 | 7.09 | 7.24 | 7.19 | 7.15 | 7.19 | 7.21 | 7.17 | 6.81 | 6.61 | --- | 6.71 | --- | 6.78 | --- | 6.88 | 6.49 | 6.86 |
| butadiene | 11Au | | R | 6.59 | 1 | 1 | 1 | 1 | 5.82 | 6.53 | 6.68 | 6.62 | 6.65 | 6.65 | 6.65 | 6.65 | 6.67 | 6.67 | 6.66 | 6.66 | 6.74 | 6.74 | 6.71 | 6.71 | 6.75 | 6.75 | 6.74 | 6.74 |
| butadiene | 21Au | | R | 6.74 | 1 | 1 | 1 | 1 | 5.89 | 6.69 | 6.88 | 6.78 | 6.80 | 6.80 | 6.80 | 6.80 | 6.83 | 6.83 | 6.83 | 6.83 | 6.87 | 6.87 | 6.85 | 6.85 | 6.89 | 6.89 | 6.88 | 6.88 |

| | Molecule | State | Flip | Rydberg | REF | n-CSF | | | | Excitation energy (eV) | | | | ASCC excitation energy (eV) | | | | | | | | PLASCC excitation energy (eV) | | | | | | | |
|---|---|---|---|---|---|---|---|---|---|---|---|---|---|---|---|---|---|---|---|---|---|---|---|---|---|---|---|---|---|
| | | | | | | *ESMF* | *CIS* | *wB97X-V* | *EOM-CCSD* | *ESMF* | *CIS* | *wB97X-V* | *EOM-CCSD* | *ESMF* | | *CIS* | | *wB97X-V* | | *EOM-CCSD* | | *ESMF* | | *CIS* | | *wB97X-V* | | *EOM-CCSD* | |
| **Medium QUEST set** | butadiene | 21Bu | Y | R | 7.87 | 1 | 1 | 1 | 1 | 7.38 | 7.83 | 7.97 | 7.93 | *8.02 | *8.01 | 7.92 | 7.92 | 7.93 | *7.93 | 7.95 | 7.96 | 7.96 | 7.96 | 7.94 | 7.94 | 7.98 | 7.98 | 7.97 | 7.97 |
| | glyoxal | 11Au | | | 2.90 | 2 | 2 | 1 | 1 | 3.26 | 3.59 | 2.85 | 3.01 | 3.13 | 3.13 | 3.14 | --- | 3.49 | 3.49 | 3.46 | 3.46 | 2.51 | 2.51 | 2.50 | 2.50 | 3.04 | 3.04 | 3.01 | 3.01 |
| | pyrrole | 11A2 | | R | 5.14 | 1 | 1 | 1 | 1 | 4.48 | 5.38 | 5.54 | 5.22 | 5.21 | 5.21 | 5.22 | 5.22 | 5.24 | 5.24 | 5.23 | 5.23 | 5.24 | 5.24 | 5.14 | 5.14 | 5.25 | 5.25 | 5.26 | 5.26 |
| | pyrrole | 21A2 | | R | 5.93 | 1 | 1 | 1 | 1 | 5.19 | 6.10 | 6.32 | 5.99 | 5.96 | 5.96 | 5.92 | 5.92 | 6.01 | 6.01 | 6.02 | 6.02 | 6.02 | 6.02 | 5.99 | 5.99 | 6.06 | --- | 6.04 | 6.04 |
| | pyrrole | 11B2 | | | 6.28 | 1 | 1 | 1 | 1 | 5.80 | 6.38 | 6.51 | 6.37 | 6.39 | 6.40 | 6.37 | 6.37 | 6.41 | 6.41 | 6.40 | 6.39 | 6.23 | 6.23 | 6.30 | 6.30 | *6.36 | *6.35 | 6.35 | 6.34 |
| | furan | 11A2 | | R | 6.00 | 1 | 1 | 1 | 1 | 5.26 | 6.04 | 6.26 | 6.07 | 6.08 | 6.08 | 6.06 | 6.06 | 6.12 | 6.12 | 6.11 | 6.11 | 6.12 | 6.12 | 6.08 | 6.08 | 6.12 | 6.12 | 6.14 | 6.14 |
| | furan | 11B2 | | | 6.39 | 1 | 1 | 1 | 1 | 6.06 | 6.37 | 6.52 | 6.53 | 6.51 | 6.51 | 6.48 | 6.48 | 6.52 | 6.52 | 6.52 | 6.53 | *6.29 | *6.31 | 6.37 | 6.37 | 6.44 | 6.44 | 6.43 | 6.44 |
| | furan | 11B1 | | R | 6.56 | 1 | 1 | 1 | 1 | 5.68 | 6.54 | 6.80 | 6.61 | 6.62 | 6.62 | 6.61 | 6.61 | 6.66 | 6.66 | 6.66 | 6.66 | 6.68 | 6.68 | 6.64 | 6.64 | 6.70 | 6.70 | 6.70 | 6.70 |
| | furan | 21A2 | | R | 6.74 | 1 | 1 | 1 | 1 | 5.91 | 6.81 | 7.06 | 6.80 | 6.78 | 6.78 | 6.76 | 6.76 | 6.81 | 6.81 | 6.83 | 6.83 | 6.85 | 6.85 | 6.79 | 6.79 | 6.76 | 6.76 | *6.87 | *6.87 |
| | furan | 21B2 | | R | 7.40 | 1 | 1 | 1 | 1 | 6.84 | 7.42 | 7.63 | 7.47 | --- | --- | --- | --- | --- | --- | --- | --- | 7.47 | 7.47 | 7.46 | 7.46 | 7.53 | 7.53 | 7.52 | 7.53 |
| | cyclopentadiene | 11B2 | | | 5.60 | 1 | 1 | 1 | 1 | 5.33 | 5.50 | 5.58 | 5.71 | 5.67 | 5.67 | 5.67 | 5.67 | 5.70 | 5.70 | 5.68 | 5.69 | 5.59 | 5.59 | 5.59 | 5.59 | 5.61 | 5.61 | 5.59 | 5.60 |
| | cyclopentadiene | 11A2 | | R | 5.70 | 1 | 1 | 1 | 1 | 4.90 | 5.71 | 5.91 | 5.74 | 5.78 | 5.78 | 5.77 | 5.77 | 5.80 | 5.80 | 5.79 | 5.79 | 5.83 | 5.83 | 5.79 | 5.79 | 5.85 | 5.85 | 5.84 | 5.84 |
| | cyclopentadiene | 11B1 | | R | 6.34 | 1 | 1 | 1 | 1 | 5.37 | 6.27 | 6.54 | 6.36 | 6.39 | 6.39 | 6.39 | 6.39 | 6.42 | 6.42 | 6.41 | 6.41 | 6.47 | 6.47 | 6.44 | 6.44 | 6.48 | 6.48 | 6.47 | 6.47 |
| | cyclopentadiene | 21A2 | | R | 6.39 | 1 | 1 | 1 | 1 | 5.50 | 6.43 | 6.67 | 6.42 | 6.43 | 6.43 | 6.41 | 6.41 | 6.46 | 6.46 | 6.45 | 6.45 | 6.51 | 6.51 | 6.47 | 6.47 | 6.52 | 6.52 | 6.52 | 6.52 |
| | cyclopentadiene | 21B2 | | R | 6.55 | 1 | 1 | 1 | 1 | 5.64 | 6.53 | 6.74 | 6.58 | 6.37 | 6.37 | 6.58 | 6.58 | --- | 6.58 | 6.57 | 6.57 | 6.65 | 6.65 | 6.63 | 6.63 | 6.68 | 6.68 | 6.67 | 6.67 |
| | thiophene | 11B2 | | | 6.06 | 1 | 1 | 1 | 1 | 5.90 | 6.06 | 6.16 | 6.20 | 6.22 | 6.22 | 6.20 | 6.20 | 6.25 | 6.25 | 6.24 | 6.23 | 6.08 | 6.08 | 6.06 | 6.06 | 6.10 | 6.10 | 6.09 | 6.09 |
| | thiophene | 11A2 | | R | 6.06 | 1 | 1 | 1 | 1 | 5.46 | 6.27 | 6.44 | 6.13 | 6.17 | 6.17 | 6.16 | 6.16 | 6.19 | 6.19 | 6.19 | 6.19 | 6.19 | 6.19 | 6.16 | 6.16 | 6.21 | 6.21 | 6.21 | 6.21 |
| | thiophene | 11B1 | | R | 6.17 | 1 | 2 | 1 | 1 | 5.76 | 6.62 | 6.59 | 6.31 | 6.40 | 6.40 | --- | --- | 6.35 | 6.35 | 6.36 | 6.36 | 5.75 | 5.75 | --- | --- | 6.30 | 6.30 | *6.37 | *6.37 |
| | thiophene | 21A2 | | | 6.31 | 1 | 1 | 1 | 1 | 6.37 | 6.73 | 6.56 | 6.37 | 6.44 | 6.44 | 6.45 | 6.45 | 6.49 | 6.49 | 6.46 | 6.46 | 6.22 | 6.22 | 6.29 | 6.29 | 6.41 | 6.41 | 6.38 | 6.38 |
| | thiophene | 21B2 | | R | 7.44 | 1 | 1 | 2 | 1 | 6.96 | 7.69 | 7.77 | 7.52 | 7.56 | 7.56 | 7.54 | 7.54 | --- | --- | 7.58 | 7.58 | 7.59 | 7.59 | 7.51 | 7.51 | --- | --- | 7.57 | 7.57 |
| | imidazole | 11A" | | R | 5.60 | 1 | 1 | 1 | 1 | 4.84 | 5.84 | 5.98 | 5.68 | 5.65 | 5.65 | 5.66 | 5.66 | 5.69 | 5.69 | 5.68 | 5.68 | 5.68 | 5.68 | 5.55 | 5.55 | 5.68 | 5.68 | 5.70 | 5.70 |
| | imidazole | 21A' | Y | | 6.43 | 1 | 1 | 1 | 1 | 6.04 | 6.73 | 6.76 | 6.58 | 6.56 | 6.68 | 6.56 | 6.66 | 6.53 | 6.72 | 6.68 | 6.55 | 5.98 | 6.44 | 6.84 | 6.93 | 6.62 | --- | 6.54 | 6.46 |
| | imidazole | 21A" | | | 6.42 | 1 | 1 | 1 | 1 | 5.53 | 6.49 | 6.72 | 6.47 | 6.40 | 6.40 | 6.34 | 6.34 | 6.46 | 6.46 | 6.47 | 6.47 | 6.49 | 6.49 | 6.45 | 6.45 | 6.53 | 6.53 | 6.51 | 6.51 |
| | benzene | 11E1g | | R | 6.46 | 1 | 1 | 1 | 1 | 5.89 | 6.60 | 6.83 | 6.49 | 6.58 | 6.58 | 6.56 | 6.56 | 6.60 | 6.60 | 6.59 | 6.59 | 6.58 | 6.58 | 6.56 | 6.56 | 6.62 | 6.62 | 6.61 | 6.61 |
| | tetrazine | 11B3u | | | 2.50 | 1 | 1 | 1 | 1 | 3.33 | 3.53 | 2.66 | 2.65 | 3.03 | 3.03 | 3.03 | 3.03 | 3.09 | 3.09 | 3.05 | 3.05 | 2.69 | 2.69 | 2.68 | 2.68 | 2.75 | 2.75 | 2.70 | 2.70 |
| | tetrazine | 11Au | | | 3.70 | 1 | 1 | 1 | 1 | 5.31 | 5.63 | 4.00 | 3.93 | 4.38 | 4.38 | 4.37 | 4.37 | 4.44 | 4.44 | 4.42 | 4.42 | 3.97 | 3.97 | 3.93 | 3.93 | 4.02 | 4.02 | 3.98 | 3.98 |
| | tetrazine | 11B2g | | | 5.50 | 1 | 2 | 1 | 1 | 6.64 | 6.79 | 5.98 | 5.88 | 6.40 | 6.40 | --- | --- | 6.46 | 6.46 | 6.41 | 6.41 | 5.54 | 5.54 | --- | --- | 5.57 | 5.57 | 5.53 | 5.53 |
| | pyridazine | 11B1 | | | 3.86 | 1 | 1 | 1 | 1 | 4.30 | 4.95 | 4.07 | 4.04 | 4.16 | 4.16 | 4.24 | 4.24 | 4.25 | 4.25 | 4.22 | 4.22 | 3.92 | 3.92 | 3.81 | 3.81 | 3.93 | 3.93 | 3.90 | 3.90 |
| | pyridazine | 11B2 | | R | 6.06 | 1 | 1 | 3 | 1 | 6.55 | 8.44 | 6.76 | 6.25 | 6.37 | 6.37 | 6.44 | 6.44 | --- | --- | 6.42 | 6.42 | 6.26 | 6.26 | *5.79 | *5.78 | --- | --- | 6.24 | 6.24 |
| | pyridazine | 21B1 | | | 6.41 | 1 | 1 | 1 | 1 | 7.48 | 8.40 | 6.69 | 6.66 | 6.91 | 6.91 | 7.01 | 7.01 | 7.01 | 7.01 | 6.98 | 6.98 | 6.60 | 6.60 | 6.48 | 6.48 | 6.62 | 6.62 | 6.60 | 6.60 |
| | cyanoacetylene | 11sig- | | | (a)5.91 | 2 | 2 | 2 | 2 | 5.02 | 5.13 | 5.28 | 6.00 | 6.19 | 6.19 | 6.20 | 6.20 | 6.22 | 6.22 | 6.20 | 6.20 | 6.19 | 6.19 | 6.08 | 6.08 | 6.13 | 6.13 | 6.10 | 6.10 |
| | cyanoacetylene | 11del | | | (a)6.17 | 2 | 2 | 2 | 2 | 5.31 | 5.42 | 5.50 | 6.25 | 6.55 | 6.55 | 6.56 | 6.56 | 6.58 | 6.58 | 6.56 | 6.56 | 6.52 | 6.52 | 6.41 | 6.41 | 6.46 | 6.46 | 6.43 | 6.43 |
| | cyanogen | 11sigu- | | | (a)6.51 | 2 | 2 | 2 | 2 | 5.43 | 5.54 | 6.09 | 6.63 | 6.84 | 6.84 | 6.85 | 6.85 | 6.87 | --- | 6.85 | --- | 6.58 | 6.58 | *6.49 | *6.47 | *6.58 | *6.58 | *6.51 | --- |
| | cyanogen | 11delu | | | (a)6.77 | 2 | 2 | 2 | 2 | 5.78 | 5.88 | 6.08 | 6.89 | 7.22 | 7.22 | 7.23 | 7.23 | 7.26 | --- | 7.24 | --- | 6.95 | 6.95 | 6.93 | 6.93 | 6.97 | --- | 6.93 | --- |
| | diacetylene | 11sigu- | | | (a)5.43 | 2 | 2 | 2 | 2 | 4.68 | 4.77 | 4.86 | 5.51 | 5.71 | 5.71 | 5.71 | 5.71 | 5.73 | 5.73 | 5.72 | 5.72 | 5.60 | 5.60 | 5.57 | 5.57 | 5.61 | 5.61 | 5.59 | 5.59 |
| | diacetylene | 11delu | | | (a)5.69 | 2 | 2 | 2 | 2 | 4.94 | 5.02 | 5.04 | 5.75 | 6.06 | 6.06 | 6.06 | 6.06 | 6.08 | 6.08 | 6.07 | 6.07 | --- | --- | --- | --- | --- | --- | --- | --- |
| | pyrazine | 11B3u | | | 4.19 | 1 | 1 | 1 | 1 | 4.94 | 5.15 | 4.36 | 4.35 | 4.70 | 4.70 | 4.71 | 4.71 | 4.75 | 4.75 | 4.72 | 4.72 | 4.32 | 4.32 | 4.33 | 4.33 | 4.38 | 4.38 | 4.34 | 4.34 |
| | pyrazine | 11Au | | | 4.98 | 1 | 1 | 1 | 1 | 6.53 | 6.95 | 5.20 | 5.19 | 5.54 | 5.54 | 5.55 | 5.55 | 5.59 | 5.59 | 5.57 | 5.57 | 5.18 | 5.18 | 5.15 | 5.15 | 5.22 | 5.22 | 5.19 | 5.19 |
| | pyrazine | 21Ag | Y | R | 6.53 | 1 | 1 | 1 | 1 | 7.64 | 8.49 | 7.09 | 6.66 | 7.04 | 7.04 | 7.04 | 7.02 | 7.08 | 7.09 | 7.06 | 7.07 | 6.82 | 6.81 | 6.76 | 6.80 | 6.85 | 6.83 | 6.83 | 6.82 |
| | pyrazine | 11B1g | | | 6.75 | 1 | 1 | 1 | 1 | 8.67 | 9.72 | 7.20 | 7.10 | 7.43 | 7.43 | 7.41 | 7.41 | 7.47 | 7.47 | 7.47 | 7.47 | 6.95 | 6.95 | *6.90 | *6.90 | 6.98 | 6.98 | 6.96 | 6.96 |
| | pyrazine | 21B1g | | R | 7.14 | 1 | 1 | 1 | 1 | 6.40 | 7.07 | 7.42 | 7.17 | 7.20 | 7.20 | 7.18 | 7.18 | 7.24 | 7.24 | 7.22 | 7.22 | 7.24 | 7.24 | 7.22 | 7.22 | 7.29 | 7.29 | 7.27 | 7.27 |
| | pyrazine | 21B2u | | R | 7.13 | 1 | 2 | 1 | 1 | 8.17 | 9.14 | 7.76 | 7.27 | 7.61 | 7.61 | --- | --- | 7.66 | 7.66 | 7.64 | 7.64 | 7.41 | 7.41 | --- | --- | 7.43 | 7.43 | 7.42 | 7.42 |
| | pyridine | 11B1 | | | 5.00 | 1 | 1 | 1 | 1 | 4.73 | 6.16 | 5.26 | 5.19 | 5.10 | 5.10 | 5.25 | 5.25 | 5.27 | 5.27 | 5.26 | 5.26 | 5.01 | 5.01 | 4.82 | 4.82 | 4.92 | 4.92 | 4.90 | 4.90 |
| | pyridine | 11A2 | | | 5.41 | 1 | 1 | 1 | 1 | 5.62 | 7.37 | 5.64 | 5.61 | 5.63 | 5.63 | 5.75 | 5.75 | 5.72 | 5.72 | 5.71 | 5.71 | 5.46 | 5.46 | 5.41 | 5.41 | 5.45 | 5.45 | 5.45 | 5.45 |

| | Molecule | State | Flip | Rydberg | REF | *n*-CSF | | | | Excitation energy (eV) | | | | ASCC excitation energy (eV) | | | | | | | | PLASCC excitation energy (eV) | | | | | | | |
|---|---|---|---|---|---|---|---|---|---|---|---|---|---|---|---|---|---|---|---|---|---|---|---|---|---|---|---|---|---|
| | | | | | | *ESMF* | *CIS* | *wB97X-V* | *EOM-CCSD* | *ESMF* | *CIS* | *wB97X-V* | *EOM-CCSD* | *ESMF* | | *CIS* | | *wB97X-V* | | *EOM-CCSD* | | *ESMF* | | *CIS* | | *wB97X-V* | | *EOM-CCSD* | |
| | pyridine | 21A2 | | R | 6.75 | 1 | 1 | 1 | 1 | 6.08 | 6.79 | 7.08 | 6.78 | 6.83 | 6.83 | 6.82 | 6.82 | 6.87 | 6.87 | 6.85 | 6.85 | 6.86 | 6.86 | 6.83 | 6.83 | 6.89 | 6.89 | 6.89 | 6.89 |
| | pyrimidine | 11B1 | | | 4.48 | 1 | 1 | 1 | 1 | 5.19 | 5.90 | 4.75 | 4.66 | 4.88 | 4.88 | 4.94 | 4.94 | 4.99 | 4.99 | 4.97 | 4.97 | 4.63 | 4.63 | 4.54 | 4.54 | 4.60 | 4.60 | 4.56 | 4.56 |
| | pyrimidine | 11A2 | | | 4.88 | 1 | 1 | 1 | 1 | 5.88 | 6.56 | 5.10 | 5.06 | 5.35 | 5.35 | 5.39 | 5.39 | 5.43 | 5.43 | 5.40 | 5.40 | 5.03 | 5.03 | 4.95 | 4.95 | 5.09 | 5.09 | 5.05 | 5.05 |
| | pyrimidine | 21B1 | | | 6.29 | 1 | 2 | 1 | 1 | 7.72 | 8.24 | 6.54 | 6.52 | 6.87 | 6.87 | --- | --- | 6.96 | 6.96 | 6.93 | 6.93 | 6.46 | 6.46 | --- | --- | 6.54 | 6.54 | 6.51 | 6.51 |
| | pyrimidine | 21B2 | | R | 6.59 | 1 | 1 | 1 | 1 | 7.33 | 8.58 | 7.21 | 6.72 | 7.03 | 7.03 | 7.07 | 7.07 | 7.11 | 7.11 | 7.07 | 7.07 | 6.86 | 6.86 | 6.56 | 6.56 | 7.08 | 7.08 | *6.83 | *6.83 |
| | triazine | 11E' | | | 7.21 | 1 | 1 | 1 | 1 | 7.86 | 9.07 | 7.70 | 7.29 | 7.63 | 7.63 | 7.63 | 7.63 | 7.69 | 7.69 | 7.68 | 7.67 | 7.44 | 7.44 | 7.43 | 7.50 | 7.50 | 7.56 | --- | 7.50 |
| Charge transfer set | ammonia-difluorine | 21A1 | | | 9.38 | 1 | 1 | 1 | 1 | 7.51 | 11.38 | 6.30 | 9.54 | 9.17 | 9.16 | 9.13 | 9.13 | 9.14 | 9.14 | 9.20 | 9.20 | 9.37 | 9.37 | 9.28 | 9.28 | 9.32 | 9.32 | 9.34 | 9.34 |
| | acetone-difluorine | 31A" | | | 5.85 | 1 | 1 | 1 | 1 | 4.17 | 8.72 | 3.70 | 6.28 | 5.74 | 5.74 | 5.77 | 5.77 | 5.74 | 5.74 | 5.84 | 5.84 | 5.85 | 5.85 | 5.79 | 5.79 | 5.81 | 5.81 | 5.87 | 5.87 |
| | pyrazine-difluorine | 21B2 | | | 6.28 | 1 | 1 | 1 | 1 | 6.42 | 9.26 | 4.35 | 6.77 | 6.51 | 6.51 | 6.42 | 6.42 | 6.48 | 6.48 | 6.56 | 6.56 | 6.47 | 6.47 | 6.33 | 6.33 | 6.43 | 6.43 | 6.48 | 6.48 |
| | pyrazine-difluorine | 21A2 | | | 6.45 | 1 | 1 | 1 | 1 | 4.83 | 7.37 | 4.41 | 6.73 | 6.41 | 6.41 | 6.36 | 6.36 | 6.37 | 6.37 | 6.72 | 6.72 | 6.58 | 6.58 | 6.36 | 6.36 | 6.62 | 6.62 | 6.53 | 6.53 |
| | ammonia_oxygendifluoride | 41A' | Y | | 7.04 | 1 | 2 | 1 | 1 | 5.41 | 9.61 | 5.11 | 7.33 | 6.95 | 6.92 | 7.56 | 7.57 | 6.95 | 6.99 | 7.08 | 7.08 | 7.01 | 6.99 | --- | --- | 6.97 | 7.07 | 6.94 | 7.00 |
| | tetrafluoroethylene-ethylene | 51B1 | | | 10.57 | 1 | 1 | 1 | 1 | 10.53 | 12.34 | 9.48 | 10.87 | 10.39 | 10.39 | 10.55 | 10.55 | 10.31 | 10.31 | 10.69 | 10.69 | 10.58 | 10.58 | 10.53 | 10.53 | --- | 10.57 | 10.68 | 10.68 |
| | 3,5-difluoro-penta-2,4-dienamine | 11A" | | | (c)6.71 | 1 | 1 | 1 | 1 | 6.44 | 8.78 | 6.68 | 7.05 | 6.84 | 6.84 | 7.07 | 7.07 | 6.98 | 6.98 | 6.96 | 6.96 | 6.76 | 6.76 | --- | --- | 6.82 | 6.82 | 6.74 | 6.74 |
